# Supplementary material for: Evaluation of a Simple, Scalable, Parallel Best-First Search Strategy
Source: arXiv:1201.3204 source file (2012-10-25)
Supplement: Supplementary file 1 [file appendix.tex]

\section*{Appendix: Differences in Planning Results Compared to Previously Reported Results}

The planning experiments described in this paper are a superset of the experiments
reported in a previous conference version of this work~\cite{ICAPS09}.
For the common part (e.g., domain-independent planning with up to 128 cores in use),
the new numerical results are slightly different from the
corresponding results in the conference paper.
This is because of a difference in HDA* implementations
as well as the nondeterministic behavior of parallel search.
Normally, checking for a duplicate state in A* is done by checking if the state is in the open/closed lists.
In the implementation of HDA* in \cite{ICAPS09}, duplicate checking was performed by checking if the
hash key of a state was present in a local open/closed list.
While the probability of a false positive duplicate detection occurring with a 64-bit hash value is quite small, the guarantee of correctness is compromised, so in this paper, our HDA* implementation checks for duplicates by comparing the actual state. This is slightly slower than checking only the hash value, but guarantees correctness.
Additionally, the Sokoban instances used in our previous work \cite{ICAPS09} were from the satisficing track of IPC-6,
while the Sokoban instances used in this paper are from the optimal track.

\section*{Appendix: Additional Tables (might not include these in final version)}

\begin{table*}[htb]
\begin{center}
\begin{scriptsize}
% [inline block 0: 7 envs, 25457 chars -> data_tex | \begin{tabular}{|@{}l@{}||c|c|c|c|c|c|c|c|} \hline...]

\caption{{\small TSUBAME2.0 24 puzzle raw runtimes}}
\end{scriptsize}
\end{center}
\end{table*}

\begin{figure}
\begin{center}
\includegraphics[width=.8\textwidth]{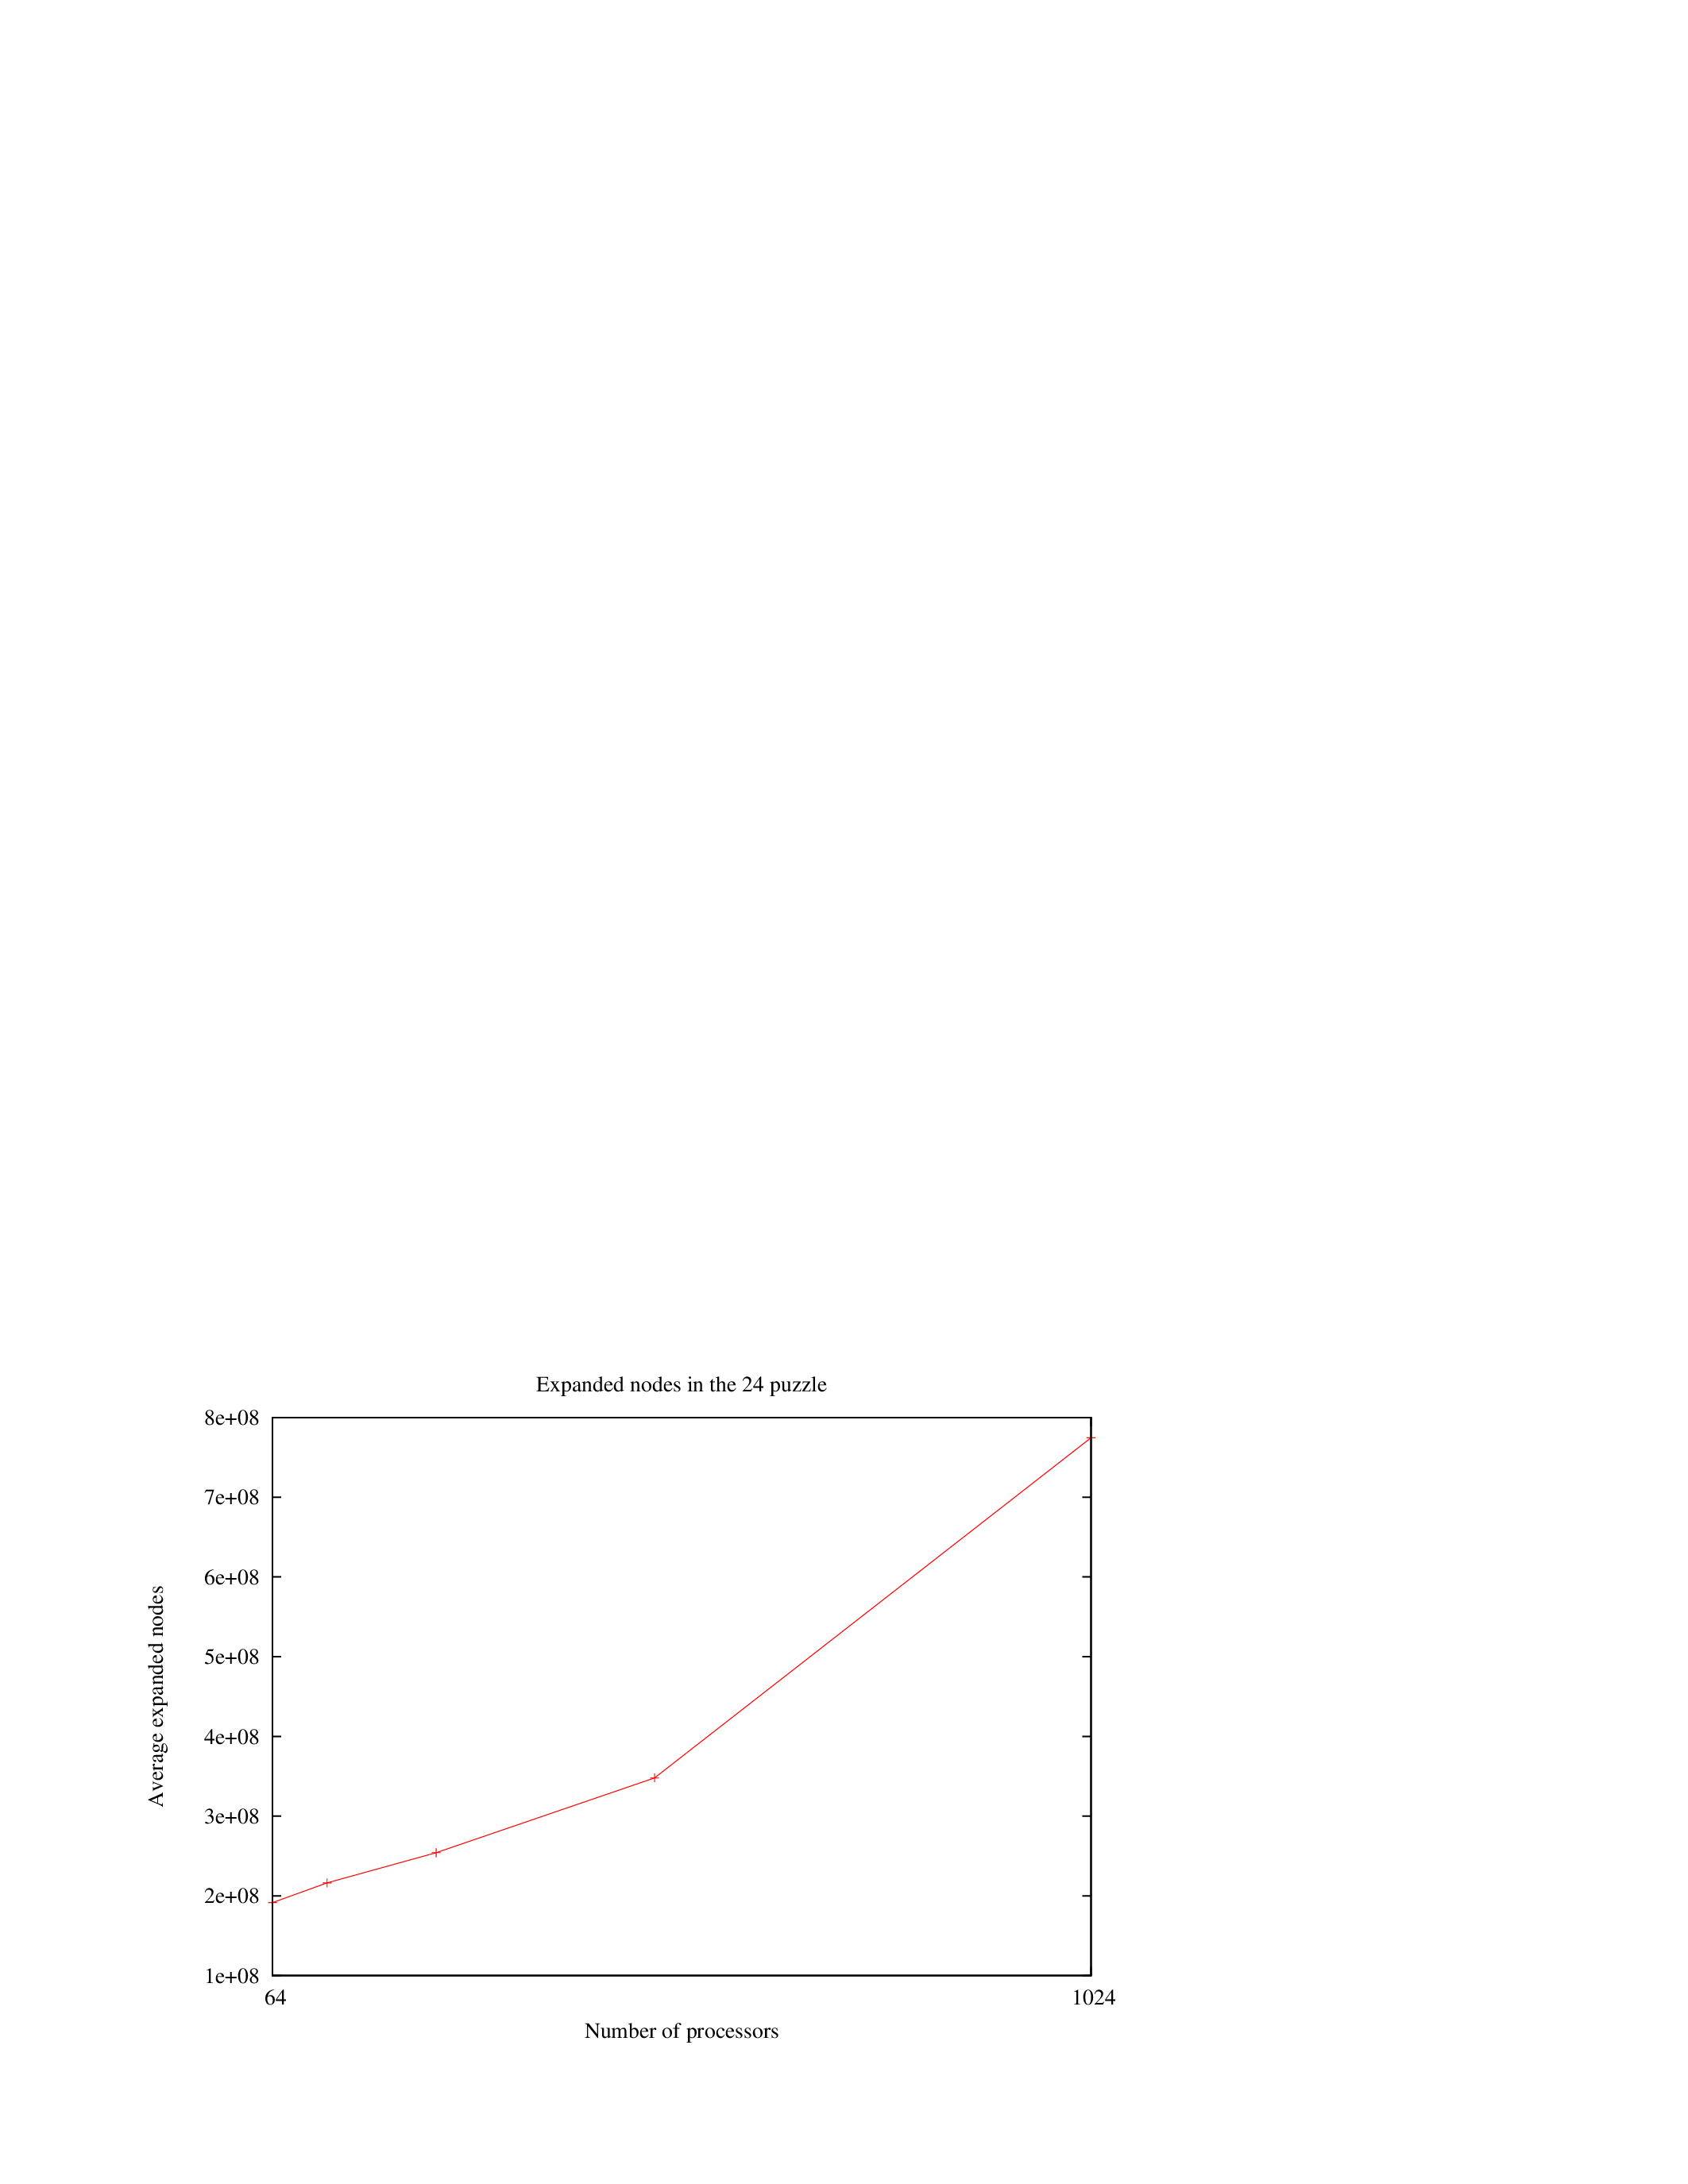}
\end{center}
\caption{{\bf TODO Update: Illustrating the growth of the search overhead in the 24 puzzle
as the number of cores increases. 
We plot the number of expanded nodes averaged over
instances solved with all 5 configurations of cores (i.e., 64, 128, 256, 512, 1024 cores). 
Experiments were performed on a HPC cluster connected by a 20Gb Infiniband network, 
where each node has eight 2.4GHz AMD dual core Opteron processors (total 16 cores per node) and 32 GB RAM. 
Kishi:  Do we really need this, since we have Table \ref{tab:tsubame2-24-puzzle-scaling-by-mincores}?
}}
\label{fig-overhead-24-puzzle}
\end{figure}

\begin{table*}[htb]
\begin{center}
\begin{scriptsize}
% [inline block 1: 6 envs, 25358 chars -> data_tex | \begin{tabular}{|@{}l@{}||c|c|c|c|c|c|c|c|c|c||@{}r@{}||@{}r@{}|}            & 12 cores  & 24 cores           & 60 cores...]

\caption{HDA* time and speed-up (between brackets) on a commodity cluster
connected by a 1Gb(x2) Ethernet network, 
where each node has two 2.33GHZ quad-core Xeon L5410 processors (total 8 cores per node) and 16GB RAM.
A machine with the same processors but with 32GB RAM was used to measure
the performance of serial A*. 
{\bf Kishi: Update the table that uses relative speedups? Numbers are available in my email sent on July 4}
}
\label{hdastar-speed-up-fun-cluster-absolute-speedup}
\end{scriptsize}
\end{center}
\end{table}

\begin{table}[htbp]
\begin{center}
\begin{scriptsize}
\begin{tabular}{|l||r|r|r|r|}
 \hline
        Instance &       A* & HDA* 16 cores  & HDA* 32 cores  & HDA* 64 cores \\
 \hline
 \hline
 \multicolumn{2}{|c|}{\bf min, avg, max speedup} & {\bf 4.1, 6.4, 9.5} & {\bf 5.3, 13.5, 20.7} & {\bf 14.3, 21.8, 31.7} \\
 \hline
        Depot10 &   17.98 ( 1.0) &  16.97 (1.06) &   8.09 (2.22) &   5.60 (3.21) \\
\hline
        Depot13 &     N/A ( N/A) & 254.41 ( 1.0) & 115.85 (2.20) &  75.09 (3.39) \\
\hline
     Driverlog8 &   17.65 ( 1.0) &  18.22 (0.97) &   7.29 (2.42) &   4.41 (4.00) \\
\hline
      Freecell5 &   20.82 ( 1.0) &  16.27 (1.28) &   8.41 (2.48) &   5.99 (3.48) \\
\hline
\hline
      Freecell7 &     N/A ( N/A) & 265.00 ( 1.0) & 128.74 (2.06) &  75.27 (3.52)\\
\hline
         Rover6 &     N/A ( N/A) &    N/A ( N/A) & 268.59 ( 1.0) & 162.82 (1.65)\\
\hline
        Rover12 &     N/A ( N/A) & 126.11 ( 1.0) &  57.66 (2.19) &  40.27 (3.13)\\
\hline
     Satellite6 &   20.00 ( 1.0) &  24.64 (0.81) &  19.86 (1.01) &   7.34 (2.72)\\
\hline
      ZenoTrav9 &   27.97 ( 1.0) &  29.87 (0.94) &  11.65 (2.40) &   7.26 (3.85)\\
\hline
     ZenoTrav11 &   79.43 ( 1.0) &  81.43 (0.98) &  32.36 (2.45) &  19.33 (4.11)\\
\hline
    PipesNoTk14 &   39.86 ( 1.0) &  34.26 (1.16) &  12.03 (3.31) &   7.86 (5.07)\\
\hline
    PipesNoTk24 &     N/A ( N/A) & 145.49 ( 1.0) &  63.31 (2.30) &  38.67 (3.76)\\
\hline
       Pegsol27 &   26.97 ( 1.0) &  22.06 (1.22) &  11.08 (2.43) &   7.43 (3.63)\\
\hline
       Pegsol28 &     N/A ( N/A) &  93.55 ( 1.0) &  45.40 (2.06) &  29.45 (3.18)\\
\hline
      Airport17 &   48.84 ( 1.0) &  33.96 (1.44) &  23.78 (2.05) &  15.99 (3.05)\\
\hline
       Gripper8 &   56.91 ( 1.0) &  53.95 (1.05) &  22.51 (2.53) &  14.97 (3.80)\\
\hline
       Gripper9 &     N/A ( N/A) & 273.47 ( 1.0) & 118.38 (2.31) &  76.39 (3.58)\\
\hline
       Mystery6 &   48.58 ( 1.0) &  39.17 (1.24) &  20.13 (2.41) &  11.91 (4.08)\\
\hline
         Truck5 &   69.40 ( 1.0) &  73.72 (0.94) &  68.71 (1.01) &  22.46 (3.09)\\
\hline
         Truck6 &     N/A ( N/A) & 675.71 ( 1.0) & 337.01 (2.01) & 168.39 (4.01)\\
\hline
         Truck8 &     N/A ( N/A) & 489.57 ( 1.0) & 284.01 (1.72) & 116.22 (4.21)\\
\hline
      Sokoban19 &   24.73 ( 1.0) &  21.10 (1.17) &  11.30 (2.19) &   9.72 (2.54)\\
\hline
      Sokoban22 &   63.65 ( 1.0) &  49.18 (1.29) &  25.20 (2.53) &  19.57 (3.25)\\
\hline
     Blocks10-2 &   50.83 ( 1.0) &  47.35 (1.07) &  20.69 (2.46) &  12.64 (4.02)\\
\hline
     Blocks12-1 &     N/A ( N/A) &    N/A ( N/A) &    N/A ( N/A) &    N/A ( N/A)\\
\hline
Logistics00-7-1 &  231.01 ( 1.0) & 230.97 (1.00) &  91.09 (2.54) &  53.37 (4.33)\\
\hline
Logistics00-9-1 &     N/A ( N/A) & 361.88 ( 1.0) & 154.09 (2.35) &  86.91 (4.16)\\
\hline
   Miconic12-2 &     N/A ( N/A) & 564.09 ( 1.0) & 259.01 (2.18) & 159.48 (3.54)\\
\hline
   Miconic12-4 &     N/A ( N/A) & 600.22 ( 1.0) & 266.08 (2.26) & 169.49 (3.54)\\
\hline
       Mprime30 &     N/A ( N/A) & 247.19 ( 1.0) & 100.27 (2.47) &  68.28 (3.62)\\
\hline
\multicolumn{5}{|c|}
{Solved only on 64 cores: Freecell6 (302.50 seconds),
Satellite7 (633.26)} \\
\multicolumn{5}{|c|}
{Sokoban26 (205.80),
Blocks11-1 (194.57) and
Logistics00-8-1 (491.02).} \\
\hline
\end{tabular}
\caption{HDA* time and speed-up (between brackets) on a commodity cluster
connected by a 1Gb(x2) Ethernet network, 
where each node has two 2.33GHZ quad-core Xeon L5410 processors (total 8 cores per node) and 16GB RAM.
A machine with the same processors but with 32GB RAM was used to measure
the performance of serial A*. 
}
\label{hdastar-speed-up-fun-cluster-sorted-by-name}
\end{scriptsize}
\end{center}
\end{table}

\begin{table*}[htb]
\begin{center}
\begin{footnotesize}
\begin{tabular}{|r|r|r|}
\hline
     16 cores &        32 cores &       64 cores   \\
\hline
     0.36\% &    0.71\% &    3.03\%  \\
\hline
\end{tabular}

\caption{Average search overhead of HDA* for instances solved by serial A* 
on a commodity cluster
connected by a 1Gb(x2) Ethernet network, 
where each node has two 2.33GHZ quad-core Xeon L5410 processors (total 8 cores per node) and 16GB RAM.
{\bf Kishi: If we use relative speedups against mincores, what should we do this this table?}
}
\label{hdastar-search-overhead-fun-cluster}
\end{footnotesize}
\end{center}
\end{table*}

\begin{table*}[htb]
\begin{center}
\begin{footnotesize}
\begin{tabular}{|r|r|r|r|r|r|}
\hline
 \multicolumn{2}{|c|}{10 states} &  \multicolumn{2}{|c|}{100 states} & \multicolumn{2}{|c|}{1000 states}  \\
 \multicolumn{1}{|c|}{spd} & \multicolumn{1}{|c|}{so} &  \multicolumn{1}{|c|}{spd} &
 \multicolumn{1}{|c|}{so} &  \multicolumn{1}{|c|}{spd} & \multicolumn{1}{|c|}{so}  \\
\hline
     15.7 & 0.53\% &    21.9 & 2.69\% &    14.1 & 17.89\%  \\
\hline

\end{tabular}
\caption{Average speedup (spd) and search overhead (so) of HDA* using 64 cores for instances solved by serial and all the HDA* versions using
64 cores\ on a commodity cluster
connected by a 1Gb(x2) Ethernet network, 
where each node has two 2.33GHZ quad-core Xeon L5410 processors (total 8 cores per node) and 16GB RAM.
{\bf Kishi: If we use relative speedups against mincores, what should we do this this table?
Should we caluclate the numbers using HDA* with 100 states as a baseline?}
}
\label{hdastar-message-pack-fun-cluster}
\end{footnotesize}
\end{center}
\end{table*}

\begin{table}[ht]
\begin{center}
\begin{footnotesize}

\begin{tabular}{|c|c|c|c|c|c|c|c|c|c|c|c|}
\hline
\multicolumn{8}{|c|}{Normal execution of HDA*}\\
\hline
            & 1 core & 64 cores & 64 cores & 64 cores & 64 cores & 64 cores & Opt \\
            & 128GB  & 4 nodes & 8 nodes  & 16 nodes & 32 nodes & 64 nodes & Len \\
\hline
{\bf Avg time} & {\bf n/a} & {\bf 117.56} & {\bf 110.88} & {\bf 93.31} & {\bf 92.28} & {\bf 87.70} & \\
\hline
Freecell7   & 2864.64 & 66.85     & 68.61     & 64.29      & 59.24      & 59.39      &  41 \\
            &         &  (42.85)  &  (41.75)  &  (44.56)   &  (48.36)   &  (48.23)   &  \\
\hline
Satellite7  & n/a     & 502.51    & 468.07    & 370.43     &  375.86    & 351.69     &  21 \\
\hline
ZenoTrav11  & 546.67  & 16.58     & 15.64     & 15.29      &  14.71     & 14.41      &  14 \\
            &         & (32.97)   &  (34.95)  &  (35.75)   &   (37.16)  &  (37.94)   &   \\
\hline
PipesNoTk24 & 1396.29 & 40.34     & 39.85     & 38.08      &  35.34     & 34.53      &  24 \\
            &         & (34.61)   & (35.04)   &  (36.67)   &   (39.51)  &  (40.44)   &   \\
\hline
Pegsol28    & 1010.65 & 21.77     & 21.31     & 20.75      &  20.47     & 19.64      &  35 \\
            &         &  (46.42)  &  (47.43)  &   (48.71)  &   (49.37)  & (51.46)    &   \\
\hline
Sokoban24   & 2635.37 & 57.29     & 51.82     & 50.99      &  48.08     & 46.51      &  205 \\
            &         &  (46.00)  &  (50.86)  &  (51.68)   &   (54.81)  &  (56.66)   &   \\
\hline
\hline
\multicolumn{8}{|c|}{HDA*, with dummy processes on cores not used by HDA*}\\
\hline
{\bf Avg time} & {\bf n/a} & {\bf 117.56} & {\bf 113.87} & {\bf n/a} & {\bf 111.31} & {\bf 113.88} & \\
\hline
Freecell7   & 2864.64 & 66.85    & 70.59    & 72.13    & 77.49    & 76.15    &  41 \\
            &         & (42.85)  & (40.58)  & (39.71)  & (36.97)  & (37.62)  &   \\
\hline
Satellite7  & n/a     & 502.51   & 466.16   & 535.86   & 445.64   & 462.22   &  21 \\
\hline
ZenoTrav11  & 546.67  & 16.58    & 21.17    & 20.15    & 19.89    & 20.54    &  14 \\
            &         & (32.97)  & (25.82)  & (27.13)  & (27.48)  & (26.61)  &   \\
\hline
PipesNoTk24 & 1396.29 & 40.34    & 44.99    & 45.26    & 43.79    & 43.80    &  24 \\
            &         & (34.61)  & (31.04)  & (30.85)  & (31.89)  & (31.88)  &  \\
\hline
Pegsol28    & 1010.65 & 21.77    & 22.88    & n/a      & 23.23    & 23.44    &  35 \\
            &         & (46.42)  & (44.17)  & n/a      & (43.51)  & (43.12)  &  \\
\hline
Sokoban24   & 2635.37 & 57.29    & 57.45    & 56.07    & 57.92    & 57.16    &  205 \\
            &         & (46.00)  & (45.87)  & (47.00)  & (45.50)  & (46.11)  &  \\
\hline
\end{tabular}
\caption{64-core scaling results with no dummy (upper half) and with dummy processes (bottom half).
Time, speedup and plan length are shown. 
Notice the increase in the average time caused by adding dummy processes.
Experiments were performed on the \tsubameone cluster.
}
\label{tab:64-core-dummy}
\end{footnotesize}
\end{center}
\end{table}
